# Supplementary material for: TCSP3.0: Template-Based Crystal Structure Prediction with Coefficient-Preserving Element Substitution and Structural Diversity
Source: arXiv:2610.34029 source file (2026-10-25)
Supplement: Supplementary file 1 [file si_labels.tex]

% generated from supplementary.aux; plain-text numbers for cross-references to the SI
\makeatletter
\expandafter\def\csname silab@sec:correctness\endcsname{S1}
\expandafter\def\csname silab@sec:original-diagnosis\endcsname{S2}
\expandafter\def\csname silab@tab:mechanisms\endcsname{S1}
\expandafter\def\csname silab@sec:ablation-details\endcsname{S3}
\expandafter\def\csname silab@tab:t800_performance\endcsname{S2}
\expandafter\def\csname silab@sec:crashfix67\endcsname{S3.2}
\expandafter\def\csname silab@tab:t800_paired\endcsname{S3}
\expandafter\def\csname silab@fig:t800_paired\endcsname{S1}
\expandafter\def\csname silab@sec:refinement\endcsname{S4}
\expandafter\def\csname silab@sec:mattersim-refinement\endcsname{S4.1}
\expandafter\def\csname silab@tab:mattersim_current\endcsname{S4}
\expandafter\def\csname silab@sec:orb-refinement\endcsname{S4.2}
\expandafter\def\csname silab@tab:orb_current\endcsname{S5}
\expandafter\def\csname silab@sec:failure-analysis\endcsname{S5}
\expandafter\def\csname silab@tab:failure_t180\endcsname{S6}
\expandafter\def\csname silab@sec:composition\endcsname{S6}
\expandafter\def\csname silab@tab:composition\endcsname{S7}
\expandafter\def\csname silab@sec:runtime\endcsname{S7}
\expandafter\def\csname silab@tab:runtime\endcsname{S8}
\expandafter\def\csname silab@sec:benchmark-inventories\endcsname{S8}
\expandafter\def\csname silab@tab:t46_inventory\endcsname{S9}
\expandafter\def\csname silab@tab:t180_inventory\endcsname{S10}
\newcommand{\siref}[1]{\ifcsname silab@#1\endcsname\csname silab@#1\endcsname\else\textbf{??}\fi}
\makeatother
